# Supplementary material for: Streamfunction-vorticity formulation for incompressible viscid and inviscid flows on general surfaces
Source: arXiv:2512.20763 ancillary file (2026-11-24)
Supplement: Supplementary file 1 [file Supplementary.pdf]

# Supplementary material

TIM BRÜERS <sup>1</sup>  
CHRISTOPH LEHRENFELD <sup>2</sup>  
MAX WARDETZKY <sup>3</sup>

<sup>1</sup> Georg August University of Göttingen, Germany  
*Email address:* t.brueers@math.uni-goettingen.de

<sup>2</sup> Georg August University of Göttingen, Germany  
*Email address:* lehrenfeld@math.uni-goettingen.de

<sup>3</sup> Georg August University of Göttingen, Germany  
*Email address:* wardetzky@math.uni-goettingen.de.

## S1. Further results and proofs

**Lemma S1.1** (Poincaré inequality). *Let  $\partial M \neq \emptyset$  and  $\Sigma$  be a portion of  $\partial M$  with strictly positive measure. Then, for any  $1 < p < \infty$ , there exists a positive constant  $C(p, \Sigma, M)$  such that every  $A \in W^{1,p}$  vanishing on  $\Sigma$  (i.e.,  $A|_{\Sigma} = 0$ ) satisfies*

$$\|A\|_{L^p} \leq C(p, \Sigma, M) \|\nabla A\|_{L^p}. \quad (\text{P}_{\leq})$$

**Proof.** This result is standard and can be found, for example, in [3, Lem I.3.1]. To prove the estimate  $(\text{P}_{\leq})$ , we argue by contradiction.

Assume the inequality does not hold. Then there exists a sequence  $A_n \in W^{1,p}$  with  $A_n|_{\Sigma} = 0$  such that  $\|A_n\|_{L^p} = 1$  and  $\|\nabla A_n\|_{L^p} < \frac{1}{n}$ . By Rellich's lemma, since the sequence is bounded in  $W^{1,p}$ , we can extract a subsequence that is Cauchy in  $\|\cdot\|_{L^p}$ . Combined with the convergence of the gradients to zero, this subsequence is Cauchy in  $\|\cdot\|_{W^{1,p}}$ . Its limit  $A \in W^{1,p}$  must satisfy  $\nabla A = 0$  and  $A|_{\Sigma} = 0$ , but  $\|A\|_{L^p} = 1$ . Since  $\nabla A = 0$  (i.e.,  $A$  is parallel) and  $M$  is connected, the scalar function  $\langle A, A \rangle$  must be constant. Because  $A$  vanishes on  $\Sigma$  (a set of strictly positive measure), this constant must be zero. Consequently,  $A = 0$  on  $M$ , which contradicts the normalization  $\|A\|_{L^p} = 1$ . ■

**Remark S1.2.** A very similar argument establishes the Poincaré inequality on  $W_0^{1,p}$  for  $1 \leq p < \infty$  in the case where  $\partial M = \emptyset$  and  $r = s = 0$ .

**Proof.** [Proof of Theorem 3.2] For bounded domains in  $\mathbb{R}^2$  and scalar functions (i.e.,  $r = 0 = s$ ), the estimate  $(\text{GN}_{\leq})$  was originally established in a generalized form in [1] and [5]. This result extends to  $(r, s)$ -tensor fields by applying the scalar estimate component-wise and using standard estimates for discrete norms.

For surfaces, we combine this Euclidean tensor estimate with a partition of unity argument. For any  $A \in \Gamma^{(r,s)}$ , this initially yields an inequality involving the full Sobolev norm

$$\|A\|_{L^p} \leq C(p, \theta, M) \left( \|A\|_{W^{1,a}}^{\theta} \|A\|_{L^a}^{1-\theta} + \|A\|_{L^a} \right).$$

Algebraic manipulations lead directly to the standard form presented in  $(\text{GN}_{\leq})$ . Since smooth sections are dense in  $W^{1,a}(\Gamma^{(r,s)})$ , the result extends to the full Sobolev space by a standard density argument. Finally, the tightened estimate  $(\text{GN}_{\leq}^0)$  is a direct consequence of the Poincaré inequality (Lemma S1.1). ■

**Proof.** [Proof of Corollary 3.4] The inclusion “ $\subset$ ” follows immediately from the Sobolev embedding theorem (Equation  $(L_{\leq}^p)$ ), Lemma 3.1 and Green's formula.

For the inclusion “ $\supset$ ”, let  $V \in L^s(\Gamma) \cap J_{L^2}$ . By definition,  $\text{div}(V) = 0$  and  $\langle V, N \rangle|_{\partial M} = 0$ . Testing the variational equation with  $\chi \in C_0^{\infty}$  implies that  $\text{curl}(V) = \omega \in L^2$ . Since  $H^1 \subset W^{1,r}$ , we may test with

arbitrary  $\chi \in H^1$ . Applying Green's formula for  $H(\text{curl})$  then yields  $\langle \langle V, T \rangle, \chi \rangle_{\partial M} = 0$ . By definition of  $H^{1/2}(\partial M)$ , this implies  $\langle V, T \rangle = 0$  in  $H^{-1/2}(\partial M)$ . Hence, Gaffney's inequality implies  $V \in H_0^1(\Gamma)$ , and thus  $V \in J_{H_0^1}$ . A final application of Green's formula, combined with the density of  $C_0^\infty$  in  $L^2$ , confirms that the equation holds for all  $\chi \in L^2$ .  $\blacksquare$

**Proof.** [Proof of  $|V|^2 \in L_T^2(W^{1,r})$  from Theorem 3.6] We begin with the case  $\partial M \neq \emptyset$ . First, we verify that  $|V|^2 \in L_T^2(L^2)$ . Since  $M$  is compact, this implies  $|V|^2 \in L_T^2(L^r)$ . Applying the Gagliardo–Nirenberg inequality (Equation (GN $_{\leq}^0$ )) with  $p = 4$  and  $a = 2$ , we estimate

$$\| |V|^2 \|_{L_T^2(L^2)} \leq C(M) \| \|\nabla V\|_{L^2} \|V\|_{L^2} \|_{L_T^2(\mathbb{R})} \leq C(M) \|V\|_{L_T^2(H^1)} \|V\|_{L_T^\infty(L^2)}.$$

Next we prove that  $\text{grad}(|V|^2) \in L_T^2(L^r)$ . Let  $s \in (2, \infty)$  be the dual exponent of  $r$  (i.e.,  $\frac{1}{s} + \frac{1}{r} = 1$ ) and choose  $q \in (2, \infty)$  such that  $\frac{1}{q} = \frac{1}{2} - \frac{1}{s}$  (which ensures  $\frac{1}{r} = \frac{1}{2} + \frac{1}{q}$ ). Applying Hölder's inequality yields

$$\| \text{grad}(|V|^2) \|_{L_T^2(L^r)} \leq 2 \| \|\nabla V\|_{L^2} \|V\|_{L^q} \|_{L_T^2(\mathbb{R})},$$

We observe that the regularity  $V \in L_T^2(J_{H_0^1}) \cap L_T^\infty(J_{L^2})$  alone is insufficient to bound the remaining term. However, we can exploit the additional regularity of  $\text{curl}(V)$  combined with Gaffney's inequality (Equation (G $_{\leq}^0$ )). Applying the Gagliardo–Nirenberg inequality (Equation (GN $_{\leq}^0$ )) with  $p = q$  and  $a = 2$  yields

$$\|V\|_{L^q} \leq C(M) \|\nabla V\|_{L^2}^{\frac{2}{s}} \|V\|_{L^2}^{1-\frac{2}{s}} \leq C(M) \|\text{curl}(V)\|_{L^2}^{\frac{2}{s}} \|V\|_{L^2}^{1-\frac{2}{s}},$$

where the second inequality follows from Gaffney's estimate. Substituting this into our previous bound, we obtain

$$\begin{aligned} \| \|\nabla V\|_{L^2} \|V\|_{L^q} \|_{L_T^2(\mathbb{R})} &\leq C(M) \left\| \|\text{curl}(V)\|_{L^2}^{1+\frac{2}{s}} \|V\|_{L^2}^{1-\frac{2}{s}} \right\|_{L_T^2(\mathbb{R})} \\ &\leq C(M) \left\| \|\text{curl}(V)\|_{L^2}^{1+\frac{2}{s}} \right\|_{L_T^2(\mathbb{R})} \|V\|_{L_T^\infty(J_{L^2})}^{1-\frac{2}{s}}. \end{aligned} \quad (\text{S1})$$

Finally, to bound the term  $\|\text{curl}(V)\|_{L^2}$ , we utilize the hypothesis  $\text{curl}(V) \in L_T^2(W^{1,r}) \cap L_T^\infty(L^r)$ . A final application of Equation (GN $_{\leq}^0$ ) with  $p = 2$  and  $a = r$  gives

$$\|\text{curl}(V)\|_{L^2} \leq C(M) \|\text{curl}(V)\|_{W^{1,r}}^{1-\frac{2}{s}} \|\text{curl}(V)\|_{L^r}^{\frac{2}{s}}.$$

Combining this inequality with (S1) yields

$$\begin{aligned} \left\| \|\text{curl}(V)\|_{L^2}^{1+\frac{2}{s}} \right\|_{L_T^2(\mathbb{R})} &\leq C(s, M) \left\| \left( \|\text{curl}(V)\|_{W^{1,r}}^{1-\frac{2}{s}} \|\text{curl}(V)\|_{L^r}^{\frac{2}{s}} \right)^{1+\frac{2}{s}} \right\|_{L_T^2(\mathbb{R})} \\ &\leq C(s, M) \left\| \|\text{curl}(V)\|_{W^{1,r}}^{1-\frac{4}{s^2}} \right\|_{L_T^2(\mathbb{R})} \|\text{curl}(V)\|_{L_T^\infty(L^r)}^{\frac{2}{s} + \frac{4}{s^2}} \\ &\leq C(s, M) \|\text{curl}(V)\|_{L_T^2(W^{1,r})}^{1-\frac{4}{s^2}} \|\text{curl}(V)\|_{L_T^\infty(L^r)}^{\frac{2}{s} + \frac{4}{s^2}}. \end{aligned}$$

This concludes the proof for the case where  $\partial M \neq \emptyset$ .

If  $\partial M = \emptyset$ , the proof proceeds analogously. The only modification required is the use of the general Gaffney inequality (Equation (G $_{<}$ )) and the general Gagliardo–Nirenberg inequality (Equation (GN $_{\leq}$ )), rather than their simplified counterparts (Equations (G $_{\leq}^0$ ) and (GN $_{\leq}^0$ )). This introduces additional terms involving  $\|V\|_{L^2}$  and  $\|\text{curl}(V)\|_{L^r}$ . However, since  $V \in L_T^\infty(J_{L^2})$  and  $\text{curl}(V) \in L_T^\infty(L^r)$ , these terms remain bounded.

Finally, we prove that  $\nabla_V V \in L_T^2(L^r(\Gamma))$ . By Lemma 3.1 (Embedding of  $W^{1,r}$ ) and the fact that  $V \in L_T^\infty(J_{L^2})$ , we deduce that the product  $\text{curl}(V)JV$  belongs to  $L_T^2(L^r(\Gamma))$ . Combining this observation

## SUPPLEMENTARY MATERIAL

with Lemma 3.5 (Nonl. term) (which relates  $\nabla_V V$  to  $\text{grad}|V|^2$  and the curl term) and the established regularity  $|V|^2 \in L_T^2(W^{1,r})$ , we conclude that  $\nabla_V V \in L_T^2(L^r(\Gamma))$ .  $\blacksquare$

**Proof.** [Proof of Proposition 2.2] The proof follows the construction in [2, p.160]. To define the pressure, we first introduce the functional  $L_t \in H^{-1}(\Gamma)$  for each  $t \in [0, T]$  by

$$\langle L_t, W \rangle := \int_0^t (\langle F_s, W \rangle - (\nabla_{V_s} V_s, W) - 2\nu(D_{V_s}, \nabla W)) ds - (V_t - V_0, W),$$

for all  $W \in H_0^1(\Gamma)$ . Using the momentum equation (Equation (NS $_{\partial_t V}$ ), or (E $_{\partial_t V}$ ) if  $\nu = 0$ ) and Green's formula, we observe that  $\langle L_t, W \rangle = 0$  whenever  $\text{div}(W) = 0$  (i.e., for all  $W \in J_{H_0^1}$ ). Consequently, by Theorem 5.3, there exists a unique scalar function  $h_t \in L_0^2$  such that  $\langle L_t, W \rangle = -(h_t, \text{div}(W))$  for all  $W \in H_0^1(\Gamma)$ . We then define the unique (distributional) pressure  $p \in (C_0^\infty(M \times (0, T)))'$  as  $p := \frac{d}{dt} h$ . A straightforward computation verifies that  $p$  satisfies Equation (P'), where the operators  $\text{grad}$ ,  $\delta$ , and  $\frac{d}{dt}$  are understood in the distributional sense. Now assume  $\partial_t V \in L_T^2(H^{-1}(\Gamma))$ . We claim that this implies  $p \in L_T^2(L_0^2)$ . To verify this, we define the functional  $\tilde{L}_t \in H^{-1}(\Gamma)$  for a.e.  $t \in (0, T)$  by

$$\langle \tilde{L}_t, W \rangle := \langle F_t - \partial_t V, W \rangle - (\nabla_{V_t} V_t, W) - 2\nu(D_{V_t}, \nabla W),$$

for all  $W \in H_0^1(\Gamma)$ . Analogous to the previous argument, the weak formulation implies that  $\langle \tilde{L}_t, W \rangle = 0$  for all  $W \in J_{H_0^1}$ . By Theorem 5.3, for a.e.  $t$ , there exists a unique  $p_t \in L_0^2$  such that  $\langle \tilde{L}_t, W \rangle = -(p_t, \text{div}(W))$ . This confirms that Equation (P) holds.

Finally, to establish that  $p \in L_T^2(L_0^2)$ , we recall that the divergence operator restricts to a topological isomorphism  $\text{div} : (J_{H_0^1})^\perp \rightarrow L_0^2$  (Theorem 5.2). Since the functional  $\tilde{L}$  belongs to  $L_T^2(H^{-1}(\Gamma))$  (following estimates similar to those in Lemma 5.1), the isomorphism property ensures that  $p$  inherits this time regularity.  $\blacksquare$

## S2. Mixed boundary conditions

In this section, we briefly derive and analyze more general mixed boundary conditions for the vorticity formulation of the Navier–Stokes equations. We accomplish this by carefully deducing the weak vorticity formulation directly from the strong velocity formulation (Equation (1.1)). For the sake of brevity, we do not address existence or regularity results for these specific boundary conditions here.

First, we must ensure that the velocity and pressure spaces are compatible. Recall that the weak pressure gradient term can be expanded as  $(\text{grad}(p), W) = -(p, \text{div}(W)) + (p, \langle W, N \rangle)_{\partial M}$ . We require that for any test function  $W$  in the homogeneous velocity space, these boundary terms vanish or are independent of the unknown pressure  $p$ . To achieve this, we partition the boundary into two disjoint admissible patches  $\partial M = \partial M_p \sqcup \partial M_N$  (following [4, Def 3.7]) and impose boundary conditions on  $p$  along  $\partial M_p$  and on the normal velocity  $\langle V, N \rangle$  along  $\partial M_N$ . Accordingly, we define the homogeneous velocity space as

$$J_{H_0^1, \partial M_N} := \{V \in H^1(\Gamma) \mid \text{div}(V) = 0, \langle V, N \rangle|_{\partial M_N} = 0\}.$$

Since the velocity space satisfies boundary conditions only on a portion of the boundary, we require a generalized Hodge decomposition to construct our vorticity formulation, analogous to Theorem 2.6. We utilize the Hodge decomposition for mixed boundary conditions from [4, Thm 4.3], which provides the following unique  $L^2$ -orthogonal decomposition

$$L^2(\Gamma) = \text{grad}(H_{0, \partial M_p}^1) \oplus \text{rot}(H_{0, \partial M_N}^1) \oplus H_{N, T}. \quad (\text{S1})$$

Here, for any admissible boundary patch  $\Sigma \subset \partial M$ , we define the potential space

$$H_{0,\Sigma}^1 := \begin{cases} \{\varphi \in H^1 \mid \varphi|_{\Sigma} = 0\} & \text{if } \Sigma \neq \emptyset, \\ H^1 \cap L_0^2 & \text{if } \Sigma = \emptyset \end{cases}.$$

The space of harmonic fields  $H_{N,T}$  is defined as

$$H_{N,T} := \{X \in H(\operatorname{div}) \cap H(\operatorname{curl}) \mid \operatorname{div}(X) = 0 = \operatorname{curl}(X), \langle Z, T \rangle|_{\partial M_p} = 0 = \langle Z, N \rangle|_{\partial M_N}\}.$$

As before,  $H_{N,T}$  is a finite-dimensional space.

Notice that if  $\partial M_N = \partial M$  (implies  $\partial M_p = \emptyset$ ), we recover the standard Hodge decomposition for  $L^2(\Gamma)$  from Theorem 3.10. Furthermore, the corresponding decomposition for  $H^k(\Gamma)$  follows from regularity results for the Laplace equation with mixed boundary conditions.

With this Hodge decomposition in hand, we derive the weak vorticity formulation from Equation (1.1) by following the steps of the symbolic proof for Theorem 2.6 (Equivalence of Navier–Stokes formulations). However, deriving the analog of Equation (NS $_{\omega}^1$ ) involves integration by parts, which introduces a new boundary term. This additional term necessitates the imposition of further boundary conditions to close the system. To address this, we again partition the boundary into two disjoint admissible patches  $\partial M = \partial M_{\omega} \sqcup \partial M_T$ , imposing boundary conditions on the vorticity  $\omega$  along  $\partial M_{\omega}$  and on the tangential velocity  $\langle V, T \rangle$  along  $\partial M_T$ .

Finally, we summarize the system incorporating all these boundary conditions. Let the boundary data  $(g_p, g_N, g_{\omega}, g_T)$  be given in the trace space  $H^{\frac{1}{2}}(\partial M_p) \times H^{-\frac{1}{2}}(\partial M_N) \times H^{\frac{1}{2}}(\partial M_{\omega}) \times H^{-\frac{1}{2}}(\partial M_T)$ , corresponding to the conditions:

$$p|_{\partial M_p} = g_p, \quad \langle V, N \rangle|_{\partial M_N} = g_N, \quad \omega|_{\partial M_{\omega}} = g_{\omega}, \quad \langle V, T \rangle|_{\partial M_T} = g_T.$$

We decompose the pressure and vorticity using liftings  $p = p_{\partial M_p} + \tilde{p}$  and  $\omega = \omega_{\partial M_{\omega}} + \tilde{\omega}$ , where  $p_{\partial M_p}, \omega_{\partial M_{\omega}} \in H^1$  satisfy the respective boundary conditions. Similarly, we decompose the velocity as  $V = V_{\partial M_N} + \tilde{V}$ . Here,  $V_{\partial M_N} := \operatorname{grad}(q)$  is defined via the unique potential  $q \in H_{0,\partial M_p}^1$  that solves the mixed boundary value problem  $\Delta_{\text{dR}} q = 0$  with  $\langle \operatorname{grad}(q), N \rangle|_{\partial M_N} = g_N$ . Applying the mixed Hodge decomposition (S1) to the remainder  $\tilde{V}$  (which has vanishing normal trace on  $\partial M_N$ ), we write  $\tilde{V} = \operatorname{rot}(\tilde{\psi}) + \tilde{H}$  with  $\tilde{\psi} \in H_{0,\partial M_N}^1$  and  $\tilde{H} \in H_{N,T}$ .

Assuming sufficient regularity for the unknowns  $\tilde{\psi}, \tilde{H}, \tilde{\omega}$ , and  $\tilde{p}$ , the system satisfies the following variational equations for a.e.  $t \in (0, T)$ :

$$\begin{aligned} (\tilde{\omega}, \chi) &= (V, \operatorname{rot}(\chi)) - (\omega_{\partial M_{\omega}}, \chi) + (g_T, \chi)_{\partial M_T}, \\ (\operatorname{rot}(\partial_t \tilde{\psi}), \operatorname{rot}(\varphi) + (\partial_t H, Z)) &= (F - \omega J V - \nu \operatorname{rot}(\omega) + 2\nu \kappa V, \operatorname{rot}(\varphi) + Z) \\ &\quad + \frac{1}{2}(|V|^2, \langle \operatorname{rot}(\varphi) + Z, N \rangle)_{\partial M_p}, \\ (\operatorname{grad}(\tilde{p}^*), \operatorname{grad}(q)) &= (F - \omega J V - \nu \operatorname{rot}(\omega) + 2\nu \kappa V, \operatorname{grad}(q)), \end{aligned}$$

for all test functions  $(\chi, \varphi, Z, q) \in H_{0,\partial M_{\omega}}^1 \times H_{0,\partial M_N}^1 \times H_{N,T} \times H_{0,\partial M_p}^1$ . In the final equation, the modified pressure is defined as  $\tilde{p}^* := \tilde{p} + \frac{|V|^2}{2} - \hat{p} \in H_{0,\partial M_p}^1$ . Here,  $\hat{p} \in H^1$  is the harmonic extension ( $\Delta_{\text{dR}} \hat{p} = 0$ ) of the boundary data  $\hat{p}|_{\partial M_p} = \frac{1}{2}|V|^2|_{\partial M_p}$  if  $\partial M_p \neq \emptyset$ , or  $\hat{p} = \frac{\|V\|_{L^2(M)}^2}{2\operatorname{Vol}(M)}$  if  $\partial M_p = \emptyset$ .

Finally, we relate the boundary conditions for  $p$  and  $\omega$  derived above to those for the Cauchy stress tensor  $\sigma(V, p) := -pI + 2\nu D_V$ , which frequently appears in velocity formulations. This relationship is established via the following identities for the deformation tensor on a admissible boundary patch  $\Sigma$ :

$$\begin{aligned} (D_V(N), W)_{\Sigma} &= \frac{1}{2}(\omega, \langle W, T \rangle)_{\Sigma} + (L_{\Sigma}(V), W)_{\Sigma}, \quad \text{if } \langle V, N \rangle|_{\Sigma} = 0 = \langle W, N \rangle|_{\Sigma}, \\ (D_V(N), W)_{\Sigma} &= (L_{\Sigma}(J V), J W)_{\Sigma}, \quad \text{if } \langle V, T \rangle|_{\Sigma} = 0 = \langle W, T \rangle|_{\Sigma}. \end{aligned}$$

## SUPPLEMENTARY MATERIAL

Here,  $L_\Sigma$  denotes the Weingarten tensor (or shape operator) of the boundary curve  $\Sigma$ , regarded as a section of  $T^{(1,1)}\Sigma$ . It is defined by  $L_\Sigma(V) := -\langle V, \nabla_T N \rangle T$ , which can be expressed in terms of the geodesic boundary curvature  $\kappa_g$  as  $L_\Sigma(V) = -\kappa_g \langle V, T \rangle T$ .

### S3. Details on numerical examples

**Schäfer Turek benchmark.** The computational domain is the rectangle with a circular obstacle, defined as  $M = [0, 2.2] \times [0, 0.41] \setminus B_{0.05}(0.2, 0.2)$ . At the inlet boundary  $\partial M_{\text{In}} = \{0\} \times [0, 0.41]$ , we prescribe a parabolic velocity profile  $V_0(y) = 4V_m y(0.41 - y)/0.41^2$  with a maximum velocity of  $V_m = 1.5$ , as illustrated in Figure 1. The flow evolution is determined by the Navier–Stokes equations with viscosity  $\nu = 0.001$  and vanishing external force ( $F = 0$ ).

Regarding boundary conditions, we impose homogeneous Dirichlet conditions ( $V = 0$ ) on the circular obstacle and the channel walls. At the outlet boundary  $\partial M_{\text{out}} = \{2.2\} \times [0, 0.41]$ , we enforce a vanishing tangential velocity  $\langle V, T \rangle = 0$  and zero pressure  $p = 0$ . Given the geometry and the condition  $\langle V, T \rangle = 0$ , this pressure condition is equivalent to  $\langle \sigma(V, p)N, N \rangle = 0$ , where  $\sigma(V, p) = -pI + 2\nu D_V$  denotes the Cauchy stress tensor, discussed in Section S2.

To address the topological complexity and the mixed boundary conditions of this benchmark, we rely on the generalized formulation derived in Section S2. This theoretical framework, based on [4], explicitly provides the machinery to realize the necessary boundary conditions for the pressure, velocity, and vorticity as discussed above.

The numerical implementation adheres to the strategy outlined in the Section 6.1. The primary adaptation involves the definition of the discrete scalar spaces: by adjusting the boundary regions where homogeneous conditions are enforced, we construct the specific discrete Hodge decomposition required for the mixed boundary constraints. Consequently, the spatial discretization and explicit Euler time integration proceed as described in Section 6.1 without further algorithmic changes.

However, enforcing the tangential boundary condition  $\langle V, T \rangle = 0$  at the outlet warrants detailed attention, particularly on coarser meshes. Due to the asymmetric positioning of the obstacle, a *Kármán vortex street* develops and convects towards the outlet (see Figure 1). Since these vortices naturally carry significant tangential velocity components, abruptly forcing  $\langle V, T \rangle$  to zero creates a strong discontinuity in the tangential velocity across the boundary elements. This, in turn, induces spurious oscillations in the vorticity field near the outlet. To mitigate these artifacts, we introduce the local  $\mathcal{O}(h^2)$  coupling term described in the main text.

Next, we introduce the quantitative metrics used to evaluate the benchmark. The problem configuration is characterized by the cylinder diameter  $L = 0.1$ . Given the kinematic viscosity  $\nu = 0.001$  and the mean inflow velocity  $V_{\text{mean}} = 1$ , the Reynolds number is  $Re = \frac{V_{\text{mean}}L}{\nu} = 100$ .

We are primarily interested in the hydrodynamic forces acting on the obstacle boundary  $\partial M_o$ . The total force is defined by the surface integral of the stress tensor,  $F_o = \int_{\partial M_o} \sigma(V, p)N ds$ . Using the no-slip condition  $V|_{\partial M_o} = 0$ , this expression simplifies to  $F_o = \int_{\partial M_o} (-pN + \nu\omega T) ds$ , where  $N$  and  $T$  denote the unit normal and tangent vectors, respectively. The drag force  $F_D$  and lift force  $F_L$  correspond to the  $x$ - and  $y$ -components of  $F_o$ . From these, the dimensionless drag and lift coefficients are derived as

$$C_D = \frac{2F_D}{V_{\text{mean}}^2 L} \quad \text{and} \quad C_L = \frac{2F_L}{V_{\text{mean}}^2 L}.$$

After an initialization period of approximately  $t = 10$ , the flow settles into a periodic regime where the lift coefficient  $C_L$  oscillates regularly. The Strouhal number is then computed from the shedding frequency  $f$  as  $St = \frac{Lf}{V_{\text{mean}}}$ .

**Kelvin–Helmholtz instability on a torus.** We define the surface  $M$  as a torus symmetric about the  $y$ -axis (lying in the  $xz$ -plane), parameterized by

$$M = \left\{ x \in \mathbb{R}^3 \mid x(\theta, \varphi) = \begin{pmatrix} (2 + \cos \varphi) \cos \theta \\ \sin \varphi \\ (2 + \cos \varphi) \sin \theta \end{pmatrix}, \theta, \varphi \in [0, 2\pi) \right\}.$$

The dynamics are driven entirely by the initial velocity  $V_0$ , which is constructed in Cartesian coordinates as

$$V_0(x, y, z) = V_\infty \tanh\left(\frac{y}{\delta_0}\right) \begin{pmatrix} z \\ 0 \\ -x \end{pmatrix} + c_n r(x, z) \exp\left(-\frac{y^2}{\delta_0^2}\right) \text{rot}(\psi_0)(x, y, z).$$

Here,  $V_\infty = 1$  denotes the reference velocity magnitude,  $\delta_0 = 0.2$  is the initial vorticity thickness, and  $c_n = 0.02$  is a noise scaling factor. The term  $r(x, z) = \sqrt{x^2 + z^2}$  denotes the radial distance in the  $xz$ -plane. Based on these parameters, the Reynolds number is computed using the characteristic length scale  $\delta_0$ , the velocity scale  $V_\infty$ , and the viscosity, yielding  $Re = \frac{\delta_0 V_\infty}{\nu} = 200$ . The perturbation is generated by the streamfunction  $\psi_0(\theta) = \cos(4\theta)$ , where  $\theta$  corresponds to the toroidal angle in the parameterization above.

## Bibliography

- [1] Emilio Gagliardo. Ulteriori proprietà di alcune classi di funzioni in più variabili. *Ricerche di Matematica*, 8:24–51, 1959.
- [2] Vivette Girault and Pierre-Arnaud Raviart. *Finite Element Approximation of the Navier-Stokes Equations*. Springer Berlin, Heidelberg, 1979.
- [3] Vivette Girault and Pierre-Arnaud Raviart. *Finite Element Methods for Navier-Stokes Equations, Theory and Algorithms*. Springer Berlin, Heidelberg, 1986.
- [4] Vladimir Gol'dshtein, Irina Mitrea, and Marius Mitrea. Hodge decompositions with mixed boundary conditions and applications to partial differential equations on lipschitz manifolds. *Journal of Mathematical Sciences*, 172(3), 2011.
- [5] L. Nirenberg. On elliptic partial differential equations. *Annali della Scuola Normale Superiore di Pisa - Scienze Fisiche e Matematiche*, Ser. 3, 13(2):115–162, 1959.
